# Supplementary material for: When Coding Style Survives Compilation: De-anonymizing Programmers from Executable Binaries
Source: arXiv:1512.08546 source file (2017-12-18)
Supplement: Supplementary file 1 [file appendix.tex]

\appendix

\begin{table}[!htbp]
\footnotesize
\begin{center}
\begin{tabular}{| p{2.2cm} |  p{1.5cm} | p{1.3cm} | p{1.3cm} |} \hline
\textbf{Feature} & \textbf{Source}&  \textbf{Number of Possible Features}  &\textbf{Information Gain Features}  \\ \hline

 {word unigrams} & hex-rays decompiled code &  29,278& 120   \\\hline
  {AST node TF*} & hex-rays decompiled code & 5,278 &  43  \\\hline
  {Labeled AST edge TF*} &  decompiled code & 26,783  & 80 \\\hline
 {AST node TFIDF**} & decompiled code & 5,278 & 37  \\\hline
 {AST node average depth} & decompiled code &5,278  & 39 \\\hline
 {C++ keywords} & decompiled code & 73 & 4 \\\hline
 radare2 disassembly unigrams & radare disassembly & 21,206 & 86  \\\hline
 radare2 disassembly bigrams &radare disassembly & 39,506 &113 \\\hline
  radare2 disassembly trigrams &radare disassembly &  112,913& 105 \\\hline
      radare2 disassembly 6-grams &ndisasm disassembly & 260,265 & 81 \\\hline

radare2 CFG node unigrams & radare disassembly & 5,297  & 13 \\\hline
radare2 CFG edges &radare disassembly & 10,246 & 5\\\hline

  ndisasm disassembly unigrams & ndisasm disassembly & 5,383  & 64   \\\hline
  ndisasm disassembly bigrams &ndisasm disassembly & 14,305  & 138 \\\hline
    ndisasm disassembly trigrams &ndisasm disassembly & 5,237 & 90\\\hline
    ndisasm disassembly 6-grams &ndisasm disassembly & 159,142 & 469\\\hline

Total & & 705,468&  1,655  \\\hline
\multicolumn{4}{|c|}{\textit{TF* = term frequency}}   \\ \hline
\multicolumn{4}{|c|}{\textit{TFIDF** = term frequency inverse document frequency}}   \\ \hline

\end{tabular}
\end{center}
\caption{ \label{tab:ig} Programming Style Features in Executable Binaries}
\end{table}
